# Supplementary material for: Effects of nucleation at a first-order transition between two superconducting phases: Application to CeRh$_2$As$_2$
Source: arXiv:2307.10374 ancillary file (2023-07-19)
Supplement: Supplementary file 1 [file Supplementary.pdf]

# Supplementary Material: Effects of nucleation at a first-order transition between two superconducting phases: Application to $CeRh_2As_2$

András L. Szabó,[1] Mark H. Fischer,[2] and Manfred Sigrist[1]

[1] *Institute for Theoretical Physics, ETH Zurich, 8093 Zurich, Switzerland*
[2] *Department of Physics, University of Zurich, 8057 Zurich, Switzerland*

In this Supplementary Material we first derive an expression for the spin currents within the Ginzburg-Landau formalism. We then elaborate on the form of the domain wall potential and present the accompanying data analysis based on numerical simulations. Finally we show the calculation of the sound absorption coefficient in details.

## S1. SPIN CURRENT

Analogously to the case of charge currents and U(1) vector potential, to compute spin currents in the Ginzburg-Landau (GL) formalism we construct an SU(2) gauge field $A^a_\mu(\boldsymbol{x})$, where $\mu = x, y$ are spatial indices and $a = x, y, z$ is the SU(2) index [1]. Due to the magnetic field aligned with $\hat{\boldsymbol{z}}$, we can single out the $A^z_\mu(\boldsymbol{x})$ component. The gauge field (an $E_u$ quantity) coupled to the spin $S_z$ (an $A_{2g}$ quantity) transforms as $E_u \otimes A_{2g} = E_u$ and with the appropriate basis vectors this object reads $\{A^z_y, -A^z_x\}$. Then, the symmetry-allowed nonvanishing term in the free energy is of the form

$$f_{\mathrm{sc}} = \sum_j \hat{D}_x A^z_y (-1)^j \epsilon(\eta^j_0 \eta^{j*}_1 + \mathrm{c.c.}),$$

with $\hat{D}_x$ the derivative operator along $x$. The spin current along $y$ is then $J^y_z = (\partial f_{\mathrm{sc}}/\partial_{A^z_y})|_{A^z_y=0}$, yielding two independent contributions localized to the DW (where the derivative is nonvanishing) as

$$J^y_z = \sum_{j=0,1} (-1)^j \epsilon \left[ L_1 \left( \frac{\partial \eta^j_0}{\partial x} \eta^{j*}_1 + \mathrm{c.c.} \right) + L_2 \left( \eta^j_0 \frac{\partial \eta^{j*}_1}{\partial x} + \mathrm{c.c.} \right) \right], \tag{S1}$$

with $L_{1,2}$ phenomenological coefficients.

## S2. DOMAIN WALL POTENTIAL

In the main text, we briefly motivate the form of the domain wall (DW) potential term in the free energy as

$$f_{\mathrm{DW}} = c(\tilde{H})\bar{x}^2 + \gamma \epsilon_{zz} \bar{x}, \tag{S2}$$

where $f_{\mathrm{DW}}$ and $\bar{x}$ are measured in units of $a_0^2/b$ and $\xi_0$, respectively, which renders the rest of the parameters dimensionless. We now proceed to elaborate on the coefficients $c(\tilde{H})$ and $\gamma$ by means of numerical simulations. The stiffness of the quadratic potential is characterized by $c(\tilde{H})$, which depends on the shape of the inhomogeneity through $\tilde{H}(x)$. To leading order, we assume its form to be $c(\tilde{H}) \propto f(w)$ with $f$ some function of $w = (\partial \tilde{H}(x)/\partial x)|_{x=0}$. For $\epsilon_{zz} = 0$, the potential minimum is located at $\bar{x} = 0$, whereas for finite strain it is shifted to

$$\bar{x} = -\frac{\gamma \epsilon_{zz}}{2c(\tilde{H})}. \tag{S3}$$

For the following analysis, we set the coupling of the order parameters to strain [Eq. (2) of the main text] to $\gamma_0 = \gamma_1 = 0.65$.

To extract the DW potential, we first use the one-step relaxed Newton-Jacobi method [2] to minimize the free energy for $\epsilon_{zz} = 0$ in the presence of a tanh-shaped inhomogeneity, centered around $\tilde{H}_t = \sqrt{a_1 - a_0}$, and with varying width $\delta$. In dimensionless form, the corresponding term in the free energy reads

$$\frac{b}{a_0^2} f_H = \left( \frac{\tilde{H}(x)}{|a_0|} \right)^2 \sum_{j=0,1} |\Psi^j_0|^2 = (1 - a_1/a_0)[1 + A \tanh(x/\delta)]^2 \sum_{j=0,1} |\Psi^j_0|^2, \tag{S4}$$

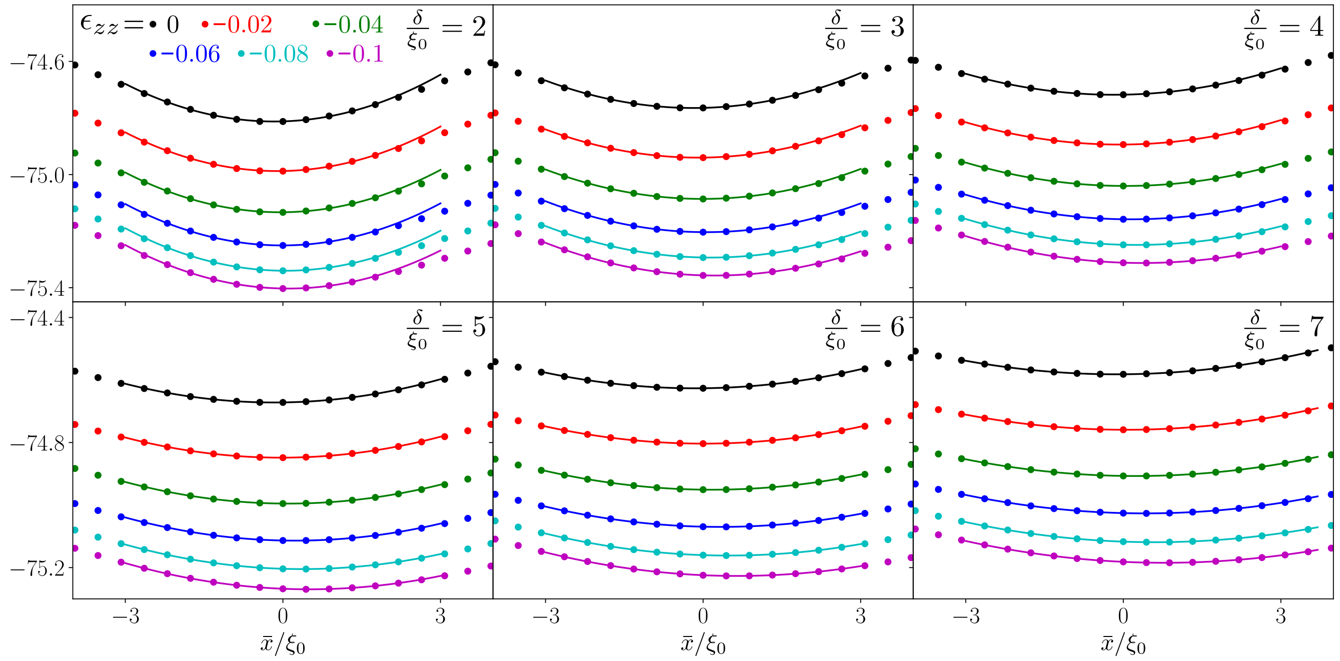


FIG. S1. DW potential (measured in units of $b/a_0^2$) for various values of $\epsilon_{zz}$ and $\delta$, with fitted parabolas for each data set. For clarity we shifted the data sets vertically in the following way: for $\epsilon_{zz} = \{0, -0.02, -0.04, -0.06, -0.08, -0.1\}$ curves are shifted by $(-1) \times \{5, 4, 3, 2, 1\}$ units of free energy, respectively.

where in the second equality we measure $\tilde{H}$ in units of $\tilde{H}_t$ and in our analysis we set the maximal deviation $A = 0.05$. The rest of the parameters are the same as in Fig. 2 of the main text. Notice that the above spatial dependence yields $w = A/\delta$. In what follows, we always use a dimensionless free energy and measure any length in units of the coherence length $\xi_0$.

As a next step, we compute the integral of the free energy density on $x/\xi_0 \in [-22, 22]$ with the previously derived numerical solution $\Psi^j_\mu(x)$ as a function of an added shift $\int \mathrm{d}x f[\Psi^j_\mu(x-\bar{x})]$ in the presence of $-0.1 \leq \epsilon_{zz} \leq 0$. However, to leading order we use the solution $\Psi^j_\mu(x)$ obtained for zero strain. To proceed and extract $c(\tilde{H})$ and $\gamma$, we fit the data obtained this way with a parabola, see Fig. S1. The fit parameters are shown in Table I.

As expected, the coefficient of the quadratic term in the fit is approximately independent of the strain, but varies strongly with $\delta$. Intuitively, the stiffness of the harmonic pinning potential is set by the inhomogeneity profile, in that slower spatial variation (larger $\delta$) yields a softer potential (smaller quadratic coefficient). Therefore, for fixed $\delta/\xi_0 = \{2, 3, 4, 5, 6, 7\}$ we average over $\epsilon_{zz}$ and notice that the function $f(w) = pw = pA/\delta$ yields an excellent fit with $p \approx 0.7$, see Fig. S2(a). Hence, we conclude that to leading order $c(\tilde{H}) \propto (\partial \tilde{H}(x)/\partial x)|_{x=0}$.

Introducing $\epsilon_{zz} > 0$ shifts the equilibrium position of the DW by an amount described by Eq. (S3). Here, $\gamma$ is independent of $\delta$, which can be seen if we shift the linear coefficients in Table I so that for $\epsilon_{zz} = 0$ the fit is purely quadratic ("corr." column). Such a correction is needed because the potential, obtained by shifting a DW solution in the expression of the free energy is necessarily slightly asymmetric, as the free energy densities of the two phases on either side of the DW are different, and we integrate them over a finite region.

To extract $\gamma$, we average over $\delta$ for each $\epsilon_{zz}$ and fit the resulting data with a linear function with zero intercept, see Fig. S2(b). This method yields $\gamma \approx 0.094$. Alternatively, $\gamma$ can be approximated via the change in energy densities of the A and B phases upon varying $\epsilon_{zz}$ as in Eq. (4) of the main text. To this end, we minimize the homogeneous free energy density $f + f_{s\eta}$ in the A and B phases separately (in the absence of DWs) for $\epsilon_{zz} = 0$. Subsequently, as before, we re-evaluate the free energy densities for varying finite strain, which yields a linear $\epsilon_{zz}$ dependence, albeit with different slopes for the A and B phases. The difference in the slopes yields $\gamma$. As reproducing this calculation is straightforward, we only quote the result $\gamma \approx 0.109$. The two scenarios therefore yield consistent values for the coupling $\gamma$.

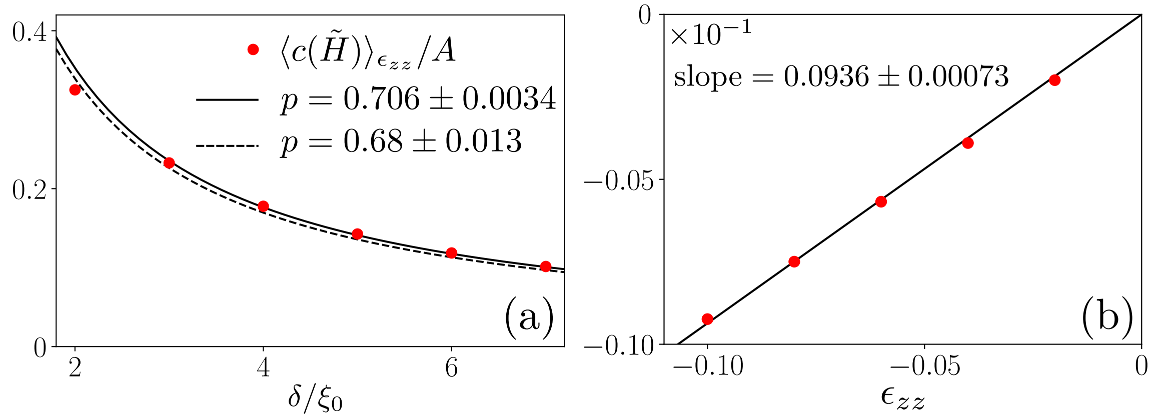


FIG. S2. (a) $c(\tilde{H})/A$ averaged over $\epsilon_{zz} = -k \cdot 0.02$ for $k = 0, 1, \ldots 5$ (red points) and least square fit of the function $p/\delta$. Dashed line represents a fit of all available data, whereas solid line ignores the first data point at $\delta = 2\xi_0$, where the inhomogeneity length scale becomes too short and our leading-order approximation is less accurate. (b) linear coefficients of the parabolic DW potential from Table I, averaged over $\delta/\xi_0 = 2, \ldots, 7$ (red points) and a linear fit with zero intercept (black line).

| $\epsilon_{zz}$ | $\delta/\xi_0 = 2$ | | | | $\delta/\xi_0 = 3$ | | | | $\delta/\xi_0 = 4$ | | | |
|---|---|---|---|---|---|---|---|---|---|---|---|---|
| | constant | linear | corr. | quadratic | constant | linear | corr. | quadratic | constant | linear | corr. | quadratic |
| 0 | -69.81 | 0.0054 | 0 | 0.0165 | -69.76 | 0.0044 | 0 | 0.0122 | -69.72 | 0.0033 | 0 | 0.0093 |
| -0.02 | -70.99 | 0.0035 | -0.0020 | 0.0163 | -70.94 | 0.0022 | -0.0022 | 0.0118 | -70.89 | 0.0013 | -0.0019 | 0.0092 |
| -0.04 | -72.13 | 0.0015 | -0.0039 | 0.0161 | -72.09 | 0.0003 | -0.0041 | 0.0117 | -72.04 | -0.0007 | -0.0039 | 0.0090 |
| -0.06 | -73.25 | 0.0004 | -0.0051 | 0.0164 | -73.20 | -0.0013 | -0.0057 | 0.0117 | -73.16 | -0.0025 | -0.0058 | 0.0088 |
| -0.08 | -74.34 | -0.0015 | -0.0069 | 0.0162 | -74.29 | -0.0032 | -0.0077 | 0.0113 | -74.25 | -0.0043 | -0.0076 | 0.0087 |
| -0.1 | -75.40 | -0.0032 | -0.0087 | 0.0160 | -75.36 | -0.0050 | -0.0095 | 0.0111 | -75.31 | -0.0061 | -0.0093 | 0.0084 |
| $\epsilon_{zz}$ | $\delta/\xi_0 = 5$ | | | | $\delta/\xi_0 = 6$ | | | | $\delta/\xi_0 = 7$ | | | |
| | constant | linear | corr. | quadratic | constant | linear | corr. | quadratic | constant | linear | corr. | quadratic |
| 0 | -69.67 | 0.0024 | 0 | 0.0074 | -69.63 | 0.0018 | 0 | 0.0062 | -69.58 | 0.0014 | 0 | 0.0053 |
| -0.02 | -70.85 | 0.0004 | -0.0020 | 0.0073 | -70.80 | -0.0001 | -0.0019 | 0.0061 | -70.76 | -0.0005 | -0.0019 | 0.0052 |
| -0.04 | -72.00 | -0.0014 | -0.0039 | 0.0072 | -71.95 | -0.0020 | -0.0038 | 0.0060 | -71.91 | -0.0024 | -0.0038 | 0.0051 |
| -0.06 | -73.11 | -0.0033 | -0.0057 | 0.0071 | -73.07 | -0.0038 | -0.0056 | 0.0059 | -73.03 | -0.0042 | -0.0056 | 0.0050 |
| -0.08 | -74.20 | -0.0051 | -0.0075 | 0.0069 | -74.16 | -0.0056 | -0.0074 | 0.0058 | -74.12 | -0.0060 | -0.0073 | 0.0050 |
| -0.1 | -75.27 | -0.0068 | -0.0092 | 0.0068 | -75.22 | -0.0073 | -0.0091 | 0.0057 | -75.18 | -0.0076 | -0.0090 | 0.0049 |

TABLE I. Fit parameters of the parabolic curves from Fig. S1, with "corr." the corrected linear coefficients, whereby all values for fixed $\delta$ are shifted by the same amount such that $\epsilon_{zz} = 0$ yields zero linear coefficient.

## S3. SOUND ABSORPTION COEFFICIENT

We first consider the equation of motion for the displacement field $u_z$ from Eq. (5) of the main text, yielding

$$\rho \partial_t^2 u_z = \partial_z \Big( \sum_{j,\mu} \gamma_\mu |\eta_\mu^j|^2 + c_{33} \partial_z u_z + \gamma \bar{x} \Big). \tag{S5}$$

In the leading-order approximation, we only consider the effect of strain on the DW via coupling to the two phases differently, and not its direct influence on the OPs. Then we obtain in Fourier space

$$-\rho \omega^2 u_z = -c_{33} k^2 u_z + ik\gamma \bar{x}. \tag{S6}$$

Next, we turn to the equation of motion of $\bar{x}$ in Eq. (5) of the main text and write it as

$$i\omega\eta\bar{x} = -c\bar{x} - ik\gamma u_z, \tag{S7}$$

and eventually we obtain

$$k = \frac{\sqrt{\rho}\omega}{\sqrt{c_{33} - \frac{\gamma^2}{i\omega\eta + c}}} \approx \frac{\sqrt{\rho}\omega}{\sqrt{c_{33}}}\left[1 + \frac{1}{2c_{33}}\frac{\gamma^2}{c + i\omega\eta}\right], \tag{S8}$$

where in the second equality we Taylor expand in $\gamma^2/[c_{33}(c + i\omega\tau)]$. Finally, we arrive at the expression for the absorption coefficient

$$\alpha = -\text{Im}\, k = \frac{\gamma^2}{2c_{33}c_s\eta}\frac{\omega^2}{\omega^2 + \omega_0^2}. \tag{S9}$$

[1] M. F. Holst, M. Sigrist, and M. H. Fischer, Role of topology and symmetry for the edge currents of a two-dimensional superconductor, Phys. Rev. Res. **4**, 013244 (2022).
[2] W. Törnig, *Eigenwertprobleme und numerische Methoden der Analysis*, Vol. 2 (Springer, Berlin, Heidelberg, 1979).
